# Supplementary material for: Comparison of Accuracy and Scalability of Gauss-Newton and Alternating Least Squares for CP Decomposition
Source: arXiv:1910.12331 source file (2020-06-10)
Supplement: Supplementary file 1 [file appendix.tex]

In this appendix, we provide additional details about our main results.

The deriviation for
\[\mat{j}^{(n p)}_{krlz} = \begin{cases}
      \displaystyle{\delta_{kl} \prod_{m=1, m\neq n}^N \Bigg(\sum_{i_m}a^{(m)}_{i_mr}a^{(m)}_{i_mz}\Bigg)}, & \text{if}\ n=p \\
      \displaystyle{a^{(n)}_{kz}a^{(p)}_{lr}\prod_{m=1, m\neq n,p}^N \Bigg(\sum_{i_m}a^{(m)}_{i_mr}a^{(m)}_{i_mz}\Bigg)}, & \text{otherwise}
    \end{cases}.\]
is as follows:

\[\mat{j}^{(n p)}_{krlz} = \displaystyle{ \sum_{i_1 \dots i_N} \Bigg(\prod_{m=1,m \neq n}^N a^{(m)}_{i_mr} \Bigg) \delta_{i_nk}   \Bigg(\prod_{m=1,m \neq p}^N a^{(m)}_{i_mz} \Bigg) \delta_{i_p l} }\]

We can combine the product for terms where $m \neq p,n$ to get

\[\mat{j}^{(n p)}_{krlz} =  \displaystyle{ \sum_{i_1 \dots i_N} \Bigg( \big(\delta_{i_n k}a^{(n)}_{i_nz}\big) \big(\delta_{i_p l} a^{(p)}_{i_pr}\big)\prod_{m=1,m \neq n,p}^N a^{(m)}_{i_mr}a^{(m)}_{i_mz} \Bigg)  }\]

Now, we can use $\sum_j\delta_{il}\delta_{lk} = \delta_{ik}$ when $n=p$,

and $\sum_l\delta_{il}a_{lk}= a_{ik}$ when $n \neq p$ to get:

\[\mat{j}^{(n p)}_{krlz} = \begin{cases}
     \delta_{kl} \sum_{i_1, \dots ,i_n}^N \Bigg(\prod_{m=1, m\neq n}^N
      a^{(m)}_{i_mr}a^{(m)}_{i_mz}\Bigg), & n=p \\
      a^{(n)}_{kz}a^{(p)}_{lr} \sum_{i_1, \dots ,i_n}^N \Bigg( \prod_{m=1, m\neq n,p}^Na^{(m)}_{i_mr}a^{(m)}_{i_mz}\Bigg)  & \text{otherwise}
    \end{cases}\]

\medskip

\linjian{Derivations for $\mat{J}^\top \mat{J} \vcr{v}$:}

{

\[\displaystyle{ \sum_{l,z} \mat{j}^{(np)}_{krlz}v_{lz}^{(p)} }  = \begin{cases}
      \displaystyle{\sum_{z}\,\Bigg(v_{kz}^{(p)}  \prod_{m=1,m \neq n}^N \Bigg(\sum_{i_m} a^{(m)}_{i_mr}  a^{(m)}_{i_mz} \Bigg) \Bigg) },   & \text{if}\ n=p  \\
      
      \displaystyle{\sum_{l,z}\,\Bigg(v_{lz}^{(p)}  a^{(n)}_{kz}a^{(p)}_{lr}\prod_{m=1, m\neq n,p}^N \Bigg(\sum_{i_m}a^{(m)}_{i_mr}a^{(m)}_{i_mz} \Bigg) \Bigg)}, & \text{otherwise}
    \end{cases}\]
}

When $n = p$,  

\es{Note that $\sum_{l}v_{lz}\delta_{kl} = v_{kz}$}

\smallskip

We can break the contractions by first computing : 

\[\prod_{m=1,m \neq n}^N \Bigg(\sum_{i_m} a^{(m)}_{i_mr}  a^{(m)}_{i_mz} \Bigg) = \Gamma^{(n,n)} \]

We save the values of $\Gamma^{(n,n)}$ during the gradient calculation and so don't have to pay for this contraction

We would now have, 

\[ \sum_{l,z} \mat{j}^{(nn)}_{krlz}v_{lz}^{(n)} = \sum_z v_{kz}^{(n)}\Gamma^{(n,n)}_{rz} \]

which would require $O(sR^2)$

\es{ For general case, this is $O(i_nR^2)$}

\medskip

Hence, the total cost is $O(sR^2)$ 

\es{ For general case, the total cost is $O\Big(\displaystyle{i_nR^2} \Big)$}

When $n \neq p$,

\[\displaystyle{\sum_{j,z}\, \mat{j}^{(np)}_{krlz}\,v_{lz}^{(p)} = \sum_{l,z}\,\Bigg(v_{lz}^{(p)}  a^{(n)}_{kz}a^{(p)}_{lr}\prod_{m=1, m\neq n,p}^N \Bigg(\sum_{i_m}a^{(m)}_{i_mr}a^{(m)}_{i_mz} \Bigg) \Bigg)  } \]

We should compute $c_{rz} = \sum_{l}v_{lz}^{(p)}a_{lr}^{(p)}$ first, which requires $O(sR^2)$

\es{General case cost $O(i_pR^2)$}

Similar to previous step, we have the value of $\Gamma^{(n,p)}$

\es{for general case cost is $O\Big(\displaystyle{(\sum_{m=1,m \neq n,p}^N i_m)R^2}\Big)$}

And then finally we can compute $\sum_{z}c_{rz}\Gamma^{(n,p)}_{rz}a_{kz}^{(n)}$ in $O(sR^2)$

\es{General cost is $O(i_nR^2)$}

\medskip

Again the total cost being $O(sR^2)$

\es{ For general case, the total cost is $O\Big((i_n +i_p)R^2\Big)$}

To compute $\displaystyle{\sum_{n=1}^N \sum_{p=1}^N \sum_{l,z} \mat{j}^{(np)}_{krlz}v_{lz}^{(p)}}$, we would need $N^2$ contractions of $\displaystyle{\sum_{l,z} \mat{j}^{(np)}_{krlz}v_{lz}^{(p)}}$ which amounts to 
$O(N^2sR^2)$

\es{For general case, $O\Big(N \displaystyle{(\sum_{m=1}^N i_m )R^2}\Big)$}
